# Supplementary material for: How to prevent type-flaw attacks on security protocols under algebraic properties
Source: arXiv:1003.5385 source file (2010-03-28)
Supplement: Supplementary file 1 [file appendix.tex]

\newpage
\noindent
{\large\bf Appendix}

\section{Unification}\label{s.defs}

\begin{definition}[Substitution]\label{d.sub}

 A \emph{substitution} $\sigma$ is denoted as $\sigma = \{ x_1/V_1,\ldots ,x_n/V_n \}$ such that $\sigma t$ represents the substitution of $x$ for all occurrences of $V$ in a term $t$ whenever $x/V \in \sigma$. 
%Further, $\forall x/V \in \sigma$, $V$ is a variable and $x$ is either a variable, ground term or a constant.

\end{definition}

\begin{definition}[Unification and unifier]~\label{d.unif}

Let $t, t'$ be two terms. Then $t,t'$ are said to be \emph{unifiable}, denoted $t \approx t'$ (read $t$ \emph{unifies with} $t'$) iff  $\sigma t = \sigma t'$ for some substitution $\sigma$; $\sigma$ is called the \emph{unifier}.  A unifier $\rho$ is called the \emph{most general unifier} (mgu) if every other unifier $\sigma$, is an extension of $\rho$; specifically $\sigma = \rho \sigma$.

\end{definition}

\section{Constraint Solving}\label{sa.prot-model}

%%%%%%%%%%%%%%%%%%%%%%%%%%%%%%%%%%%%%%%%%%%%%%%%%%%%%%%%%%%%%%%%%%%%
%%%%%%%%%%%%  Reduction Procedure, P [MS01]   %%%%%%%%%%%%%%%%%%%%%%
%%%%%%%%%%%%%%%%%%%%%%%%%%%%%%%%%%%%%%%%%%%%%%%%%%%%%%%%%%%%%%%%%%%%

\subsection{Constraint Satisfaction Procedure \textbf{P}~\cite{MS01}}\label{ssa.redn-proc}

\begin{center}
 \begin{tabbing}
  \= ~~~$C :=$~initial constraint sequence \\
  \> ~~~$\sigma := 0$ \\
  \> ~~~\texttt{repeat} \\
  \> ~~~~~~ \texttt{let} $c^* = m : T$ be \= the constraint in $C$ \\
  \> \>  s.t. $m$ is not a variable \\
  \> ~~~~~~ \texttt{if} $c^*$ \= not found \\
  \> \> \texttt{output} \textbf{Satisfiable!} \\
  \> ~~~~~~apply rule \textit{(elim)} to $c^*$ until no longer applicable \\
  \> ~~~~~~$\forall r \in R$ \\
  \> ~~~~~~~~~\texttt{if} $r$ \= is applicable to $C$ \\
  \> \> $\langle C';\sigma'\rangle := r(C;\sigma)$ \\
  \> \> create node with $C'$; add $C \to C'$ edge \\
  \> \> push $\langle C'; \sigma' \rangle$ \\
  \> ~~~~~~~~~$\langle C;\sigma\rangle :=$ \texttt{pop} \\
  \> ~~~\texttt{until emptystack}  
 \end{tabbing}
\end{center}
